# Supplementary material for: Coupled Interfacial Phenomena Suppress Propulsion in Catalytic Janus Colloids
Source: arXiv:2509.14471 source file (2025-09-28)
Supplement: Supplementary file 1 [file Coupled_Interfacial_SI.pdf]

## Supplementary Information

Sulfate latex polystyrene particles (3  $\mu\text{m}$  diameter, 8% wt./vol) were purchased from Fisher Scientific (Lot # 2855924). The original particle suspension was sonicated for 30 minutes before extracting 1.5 mL into a separate vial. This sample was centrifuged (Thermo Scientific, SORVALL LEGEND MICRO CENTRIFUGE) at 2000 rpm for 30 minutes to sediment the particles. The supernatant was carefully removed and replaced with fresh ultra-pure water (18.2 M $\Omega$ ) generated from Arium Mini Ultrapure Water Systems (Sartorius, USA) . This washing process was repeated five times. A final concentration of 9% wt./vol was prepared, which was found to yield optimal monolayer of polystyrene particles on wafer surface. A 20 mm  $\times$  20 mm silicon wafer was plasma-cleaned for 2 minutes and placed in a spin coater (Ossila). A 20  $\mu\text{L}$  aliquot of the particle suspension was deposited onto the wafer, and the spin coating was performed in two steps: 500 rpm for 5 seconds, followed by 6000 rpm for 30 seconds. The resulting monolayers were examined under an Olympus BX51WI microscope at 40 $\times$  magnification. The wafers were then affixed to glass slides using thermal tape and stored in petri dishes for subsequent platinum deposition. Platinum layers of 3 nm, 7nm, 10 nm, 20 nm, and 35 nm thickness were deposited onto the monolayers using Physical Vapor Deposition (Angstrom Engineering Evovac Deposition System ). The deposition rate was maintained at 2  $\text{\AA}/\text{sec}$ .

Individual wafers containing Janus particles were submerged in ultra-pure water within a 50 mL centrifuge tube and sonicated for 1–2 hours to detach the particles into suspension. The suspension was then divided into multiple 1.5 mL vials and centrifuged at 4000 rpm for 15–20 minutes to pellet the particles. The supernatant was carefully removed, and the pellet was re-suspended in fresh ultra-pure water. This washing process was repeated five times to remove residual contaminants. A dilute working solution was prepared by diluting 10  $\mu\text{L}$  of the concentrated suspension in 1000  $\mu\text{L}$  ultra-pure water. This allowed observing particles in single particle domain, without

interactions with other particles. The particles were observed under a  $20\times$  objective to ensure an optimal density of  $\sim 10$  particles per field of view ( $341\ \mu\text{m} \times 408\ \mu\text{m}$ ). This ensured that particles did not have any interaction with each other.

For plasma cleaning, glass slides were cleaned sequentially in an IPA solution (sonication, 15 minutes), rinsed with ultra-pure water, dried with compressed air, and further cleaned in acetone (sonication, 15 minutes). The slides were then subjected to plasma cleaning (Tergeo Plasma Cleaner, 2 minutes, air plasma) to render the surface hydrophilic and negatively charged. Immediately after plasma cleaning, a secure seal spacer was placed onto the slide, and  $7\ \mu\text{L}$  of Janus particle suspension containing hydrogen peroxide at the required concentration was added. The inner lining of the spacer was marked with a hydrophobic pen (VWR Technologies) to prevent loss of water through pores and thus prevent convection. The well was sealed with a coverslip to prevent evaporation, and the assembled fluid cell was transferred to the microscope for observation. Untreated glass slides were used directly from the packaging of premium glass slides.

Particles were recorded immediately upon setting the fluid cell. The microscope focus was adjusted to capture particles at the lowest and highest available plane, ensuring proximity to the boundaries of glass slide (bottom) and cover slip (top). Video recordings were conducted using a  $20\times$  objective at 10 fps for 100 seconds per field of view using digital camera (ThorLabs). Videos were recorded up to 20 minutes from setting fluid cell, with alternating 100 seconds videos between bottom and top boundary within each fluid cell, avoiding regions near bubbles or cell edges. If ceiling state particles were not found, flooring was recorded. Three repetitions of fluid cells for each condition were performed. Videos were stored as .avi files for further processing.

ImageJ software with the TrackMate plugin was used to extract particles' tracks information. A custom made Jython script automated the process by converting .avi files to 8-bit grayscale TIFF images, applying binary and Gaussian blur filters to enhance particle identification, and detecting particle centers and generating XML files containing (t, x, y) coordinates for each track. The mean squared displacement (MSD) was calculated and the equation  $\text{MSD} = 4D\tau + v^2\tau^2$  was used for fitting, where  $D$  is the diffusion coefficient,  $v$  is the velocity, and  $\tau$  is the time interval. MSD fitting of  $\tau = 1$  seconds (10 frames) was used for 100 seconds (1000 frames) videos to capture the activity in the MSD. Maximum displacement of trajectory of particle is

defined to be the maximum linear distance between any two points on the track. Mean of values for each condition and their standard deviation was plotted on Origin. Trajectories of particles centered at (0,0) for comparison were plotted using a python code.

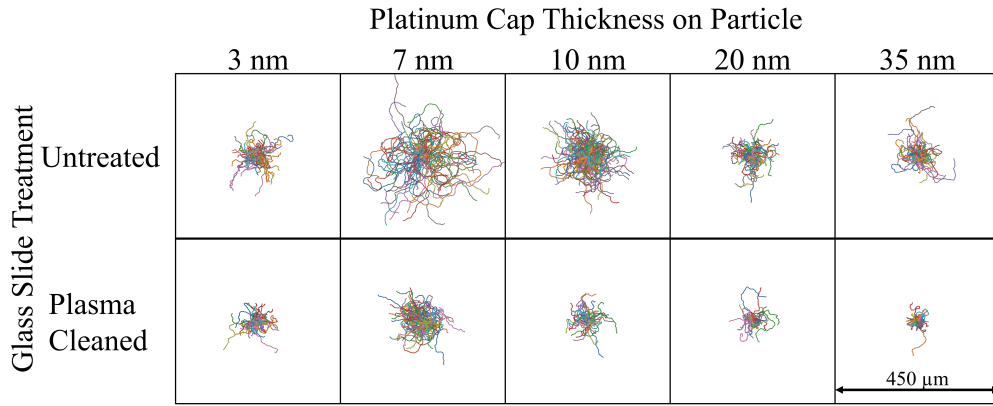

Figure 1: Trajectories of all ceiling and flooring particles in 3 wt./vol % hydrogen peroxide solution on untreated and plasma cleaned boundaries. Different colors represent different particles. Each trajectory is 100 seconds long.

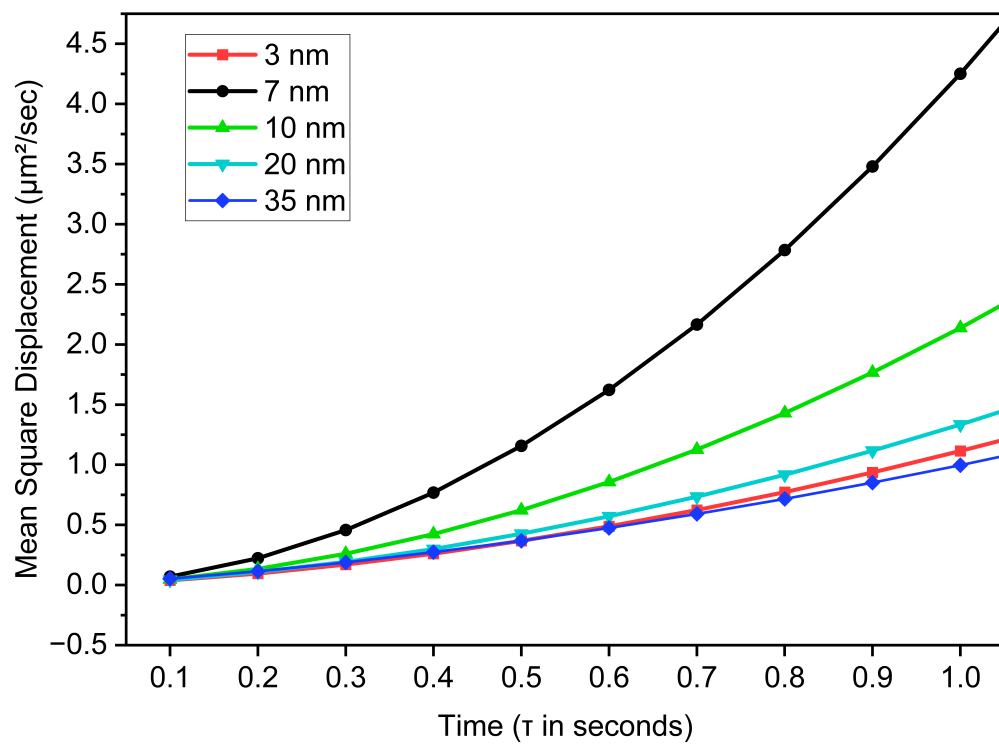

Figure 2: Mean squared displacement of Janus particles with different cap thickness in 3 wt./vol % hydrogen peroxide in water solution. Average mean square displacement of five flooring particles closest to average velocity is shown for each particle cap thickness.
